# Supplementary material for: Earthquake theorem for cluster algebras of finite type
Source: arXiv:2206.15226 source file (2024-12-13)
Supplement: Supplementary file 1 [file 8_appendix.tex]

\appendix

\section{Non-positivity of the product of $C$- and $F$-matrices}\label{app:non-positive}

\begin{defi}[{\cite{FuGy}}]\label{def:F-mat}
We fix $v_0 \in \bExch_\bs$.
For each $i, j \in I$ and $v \in \bExch_\bs$, let $f_{ij}$ denote the maximal degrees of $X_j$ in the $i$-th $F$-polynomial $F^{v_0 \to v}_i(X^0_1, \dots, X^0_n)$.
Then
% $\mathbf{f}_i^{(t)}:= (f^{(t)}_{i1}, \dots, f^{(t)}_{iN})$ is called the $f$-vector and 
$F^{\bs}_{v_0 \to v} := (f_{ij})_{i,j \in I}$ is called the \emph{$F$-matrix} from $v_0$ to $v$ in $\bs$.
\end{defi}

\begin{defi}
\begin{enumerate}
    \item Let $\gamma$ be a path
    \begin{align*}
        \gamma: v_0 \overbar{k_0} v_1 \overbar{k_1} \cdots \overbar{k_{m-1}} v_m = v
    \end{align*}
    in $\bExch_\bs$ and $(i(0), i(1), \dots, i(\ell-1))$ denotes the subsequence of $(0, 1, \dots, m-1)$ such that $v_{i(t)} \overbar{k_{i(t)}} v_{i(t)+1}$, $t=0, 1, \dots, \ell-1$ are the horizontal edges of $\gamma$.
    Take the tuple $\mathbf{\epsilon}^\trop_\gamma = (\epsilon_0, \dots, \epsilon_{\ell-1})$ of tropical signs of the $k_{i(t)}$-th $c$-vector from $v_0$ to $v_{i(t)}$.
    We call it also \emph{tropical sign} of the path $\gamma$.
    \item A path $\gamma: v_0 \to v$ in $\bExch_\bs$ is \emph{weakly green} if its tropical sign $\boldsymbol{\epsilon}^\trop_\gamma = (\epsilon_{0}, \dots, \epsilon_{\ell -1})$ and the tropical sign $\boldsymbol{\epsilon}^\trop_{-\gamma} = (\overline{\epsilon}_{0}, \dots, \overline{\epsilon}_{\ell-1})$ of the path $-\gamma: -v \to -v_0$ in $\bExch_{-\bs}$ corresponding to $\gamma$ satisfy $(\epsilon_k, \overline{\epsilon}_k) = (+,+)$, $(+,-)$ or $(-,+)$ for any $k=0, \dots, \ell-1$
\end{enumerate}
\end{defi}

\begin{thm}\label{thm:FC_non-pos}
Let $\bs$ be a mutation class and $v_0, v \in \bExch_\bs$.
If there is a weakly green path $\gamma: v_0 \to v$ in $\bExch_\bs$,
% with the tropical signs $\boldsymbol{\epsilon}^\trop_\gamma = (\epsilon_{\ell-1}, \dots, \epsilon)$, $\boldsymbol{\epsilon}^\trop_{-\gamma} = (\overline{\epsilon}_{\ell-1}, \dots, \overline{\epsilon}_0)$ are satisfying $(\epsilon_k, \overline{\epsilon}_k) = (+,+)$ $(+,-)$ or $(-,+)$ for $k={\ell-1}, \dots, 0$.
then the products $F^\bs_{v \to v_0} C^{\pm \bs}_{v_0 \to v}$ are non-positive matrices.
% Here, $-\gamma: -v \to -v_0$ be a path in $\bExch_{-\bs}$ corresponding to $\gamma$.
\end{thm}

By \cite{AIR}, if $\bs$ be of finite type, then there is a path $\gamma: v_0 \to v$ with $\boldsymbol{\epsilon}^\trop_\gamma = (+, \dots, +)$ for any vertices $v_0, v \in \bExch_\bs$.
(See also \cite[Theorem 3.6]{BY}.)
Thus, we have the following:
\begin{cor}\label{cor:FC_non-pos_fin}
If $\bs$ be of finite type, then the products $F^\bs_{v \to v_0} C^{\pm \bs}_{v_0 \to v}$ are non-positive matrices for any $v_0, v \in \bExch_\bs$.
\end{cor}

The mutation class $\bs$ with an initial seed
\begin{align*}
    \bigg(
    \begin{pmatrix}
    0 & \ell\\
    -\ell & 0
    \end{pmatrix},\ 
    (X^0_1, X^0_2)
    \bigg)
\end{align*}
is called \emph{$\ell$-Kronecker} mutation class for $\ell \geq 2$.
It is well-known that the graph $\bExch_\bs$ is ladder graph of infinite length:
% , looks like the following:
\[
\begin{tikzcd}
\cdots \ar[r, no head, "2"] & v_{-2} \ar[r, no head, "1"] \ar[d, no head, "(1\ 2)"] & v_{-1} \ar[r, no head, "2"] \ar[d, no head, "(1\ 2)"] & v_0 \ar[r, no head, "1"] \ar[d, no head, "(1\ 2)"] & v_1 \ar[r, no head, "2"] \ar[d, no head, "(1\ 2)"] & v_2 \ar[r, no head, "1"] \ar[d, no head, "(1\ 2)"] & \cdots\\
\cdots \ar[r, no head, "1"] & v'_{-2} \ar[r, no head, "2"] & v'_{-1} \ar[r, no head, "1"] & v'_0 \ar[r, no head, "2"] & v'_1 \ar[r, no head, "1"] & v'_2 \ar[r, no head, "2"] & \cdots
\end{tikzcd}
\]

In particular, infinite paths
Let us consider the infinite paths:
\begin{align*}
    \gamma^\infty&: v_0 \overbar{1} v_1 \overbar{2} v_2 \overbar{1} v_3 \overbar{2} \cdots,\\
    \gamma^{-\infty}&: v_0 \overbar{2} v_{-1} \overbar{1} v_{-2} \overbar{2} v_{-3} \overbar{1} \cdots.
\end{align*}
By the direct calculation, we can verify that
\begin{align*}
    \boldsymbol{\epsilon}_{\gamma^\infty}^\trop &= (+, +, -, -, -, \dots),\\
    \boldsymbol{\epsilon}_{\gamma^{-\infty}}^\trop &= (+, +, +, +, +, \dots).
\end{align*}
Also, we note that the cluster modular group $\Gamma_\bs$ of the $\ell$-Kronecker mutation class isomorphic to $\bZ$ and the generator $\phi$ of it is given by the path
\begin{align*}
    \gamma: v_0 \overbar{1} v_1 \overbar{(1\ 2)} v'_1.
\end{align*}
By the sign stability of $\phi$ (resp. $\phi^{-1}$) \cite[Example 5.3]{IK21}, the sign $\boldsymbol{\epsilon}_{\gamma^{\infty}}^\trop$ (resp. $\boldsymbol{\epsilon}_{\gamma^{-\infty}}^\trop$) consists of only minus except for first two components (resp. only plus) since $\gamma^\infty$ (resp. $\gamma^{-\infty}$) represents the iteration $\phi^\infty$ (resp. $\phi^{-\infty}$) infinite times.
Therefore, any two vertices $v_0, v \in \bExch_\bs$ are connected by weekly green paths.
\begin{cor}
Let $\bs$ be an $\ell$-Kronecker mutation class for $\ell \geq 2$.
Then, the products $F^\bs_{v \to v_0} C^{\pm \bs}_{v_0 \to v}$ are non-positive matrices for any $v_0, v \in \bExch_\bs$.
\end{cor}

We think this phenomena for all mutation class.
\begin{conj}\label{conj:FC_nonpos}
Let $\bs$ be a mutation class and $v_0, v \in \bExch_\bs$.
Then, there is a weekly green path from $v_0$ to $v$.
In particular, the products $F^\bs_{v \to v_0} C^{\pm \bs}_{v_0 \to v}$ are non-positive matrices.
\end{conj}

For the proof of \cref{thm:FC_non-pos}, we define the notation:
for $v \in \bExch_\bs$, $k \in I$ and a sign $\epsilon \in \{+,-\}$, the matrices $E^{(v)}_{k,\epsilon} = (E_{ij})_{i,j \in I}$ are given by
\begin{align*}
    E_{\indi\indj}:=
    \begin{cases}
        1 & \mbox{if $i=j \neq k$}, \\
        -1 & \mbox{if $i=j=k$}, \\
        [\epsilon \cdot \ve_{ik}^{(v)}]_+ & \mbox{if $j = k$ and $i \neq k$}, \\
        0 & \mbox{otherwise}.
    \end{cases}
\end{align*}

\begin{proof}[Proof of \cref{thm:FC_non-pos}]
Let us take a weakly green path 
\begin{align*}
    \gamma: v_{0} \overbar{k_{0}} v_1 \overbar{k_1} \cdots \overbar{k_{\ell-2}} v_{\ell-1} \overbar{k_{\ell-1}} v_\ell = v
\end{align*}
and we suppose that it is horizontal for simplicity.
We put $v' := v_{\ell-1}$, $k := k_{\ell-1}$.
% in $\bExch_\bs$ satisfying the condition of the tropical signs in \cref{thm:FC_non-pos}.
By \cite[Proposition 3.9 (2)]{FuGy}, we have
\begin{align}
    F^\bs_{v \to v_0} 
    &= F^\bs_{v' \to v_0} E^{(v)}_{k, \epsilon} + [\epsilon G^\bs_{v' \to v_0}]_+^{\bullet k}\label{eq:F_rear_bs}\\
    &= F^\bs_{v' \to v_0} E^{(-v)}_{k, \oline{\epsilon}} + [\oline{\epsilon} G^{-\bs}_{v' \to v_0}]_+^{\bullet k}.\label{eq:F_rear_-bs}
\end{align}
Here,
\begin{itemize}
    \item $\epsilon$ and $\overline{\epsilon}$ are the $\ell$-th component of the tropical sign of $\gamma$ and $-\gamma$, respectively and
    \item for a matrix $A$, $A^{\bullet k}$ denotes the product $A \cdot \mathrm{diag}(0,\dots,0,\overset{k}{1},0,\dots,0)$ and $[A]_+$ is the matrix obtained by applying $[-]_+$ to each entries.
\end{itemize}
We note that $\epsilon G^{-\bs}_{v' \to v_0} \mathbf{e}_{k} \in \bZ_{\geq 0}^I \Leftrightarrow \epsilon (C^{\bs}_{v_0 \to v'})^\tr \mathbf{e}_{k} \in \bZ_{\geq 0}^I$ and $\overline{\epsilon} G^{\bs}_{v' \to v_0} \mathbf{e}_{k} \in \bZ_{\geq 0}^I \Leftrightarrow \overline{\epsilon} (C^{-\bs}_{v_0 \to v'})^\tr \mathbf{e}_{k} \in \bZ_{\geq 0}^I$ by \cref{thm:C-mat} (2).
Moreover, by \cite[Proposition 1.3]{NZ}, we have
\begin{align}
    C^{\bs}_{v_0 \to v} &=
    E^{(v)}_{k, \epsilon} C^\bs_{v_0 \to v'}\label{eq:C_front_bs}\\
    C^{-\bs}_{v_0 \to v} &=
    E^{(-v)}_{k, \overline{\epsilon}} C^{-\bs}_{v_0 \to v'}.\label{eq:C_front_-bs}
\end{align}
% Using \eqref{eq:F_rear_bs}, \eqref{eq:C_front_bs} and
Since $(E^{(v)}_{k, \epsilon})^2 = \mathrm{Id}$, 
\begin{align}
    \quad F^\bs_{v \to v_0} C^{\bs}_{v_0 \to v} &= 
    F^\bs_{v' \to v_0} C^{\bs}_{v_0 \to v'} + [\epsilon G^{\bs}_{v' \to v_0}]_+^{\bullet k} C^{\bs}_{v_0 \to v} \quad\mbox{(by \eqref{eq:F_rear_bs} and \eqref{eq:C_front_bs})},\label{eq:FC_decomp_bs}\\
    % &= F^\bs_{v' \to v_0} C^{\bs}_{v_0 \to v'} + [\epsilon (C^{-\bs}_{v_0 \to v'})^\tr]_+^{\bullet k} C^{\bs}_{v_0 \to v},\\
    \quad F^\bs_{v \to v_0} C^{-\bs}_{v_0 \to v} &= 
    F^\bs_{v' \to v_0} C^{-\bs}_{v_0 \to v'} + [\overline{\epsilon} G^{-\bs}_{v' \to v_0}]_+^{\bullet k} C^{-\bs}_{v_0 \to v} \quad\mbox{(by \eqref{eq:F_rear_-bs} and \eqref{eq:C_front_-bs})}.\label{eq:FC_decomp_-bs}
    % &= F^\bs_{v' \to v_0} C^{-\bs}_{v_0 \to v'} + [\overline{\epsilon}_0 (C^{\bs}_{v_0 \to v'})^\tr]_+^{\bullet k} C^{-\bs}_{v_0 \to v}.
\end{align}
We put $C^\bs_{v_0 \to v'} = (c_{ij})_{i,j \in I}$, $C^{-\bs}_{v_0 \to v'} = (\oline{c}_{ij})_{i,j \in I}$, $C^\bs_{v_0 \to v} = (c'_{ij})_{i,j \in I}$ and $C^{-\bs}_{v_0 \to v} = (\oline{c}'_{ij})_{i,j \in I}$.
Then, 
\begin{align}
    [\epsilon G^{\bs}_{v' \to v_0}]_+^{\bullet k} C^{\bs}_{v_0 \to v} &= [\epsilon D(C^{-\bs}_{v_0 \to v'})^\tr D^{-1}]_+^{\bullet k} C^{\bs}_{v_0 \to v}\nonumber\\
    &= ([\epsilon d_i \oline{c}_{ki} d_{k}^{-1}]_+ c'_{kj})_{i,j \in I}
    = \begin{cases}
        (-\epsilon d_i d_{k}^{-1} \oline{c}_{k i} c_{k j})_{i,j \in I} & \mbox{if } \epsilon \oline{\epsilon} = +,\\
        O & \mbox{if } \epsilon \oline{\epsilon} = -.
    \end{cases}\label{eq:[C]C_bs}\\
    [\overline{\epsilon} G^{-\bs}_{v' \to v_0}]_+^{\bullet k} C^{-\bs}_{v_0 \to v} &=
    [\epsilon D(C^{\bs}_{v_0 \to v'})^\tr D^{-1}]_+^{\bullet k} C^{-\bs}_{v_0 \to v}\nonumber\\
    &= ([\oline{\epsilon} d_i {c}_{k i} d_{k}^{-1}]_+ \oline{c}'_{kj})_{i,j \in I}
    = \begin{cases}
        (- \oline{\epsilon} d_i d_{k}^{-1} {c}_{ki} \oline{c}_{kj})_{i,j \in I} & \mbox{if } \epsilon \oline{\epsilon} = +,\\
        O & \mbox{if } \epsilon \oline{\epsilon} = -.
    \end{cases} \label{eq:[C]C_-bs}
    %  \begin{cases}
    %     (0, \dots, 0,\overline{\mathbf{c}}_{k}^\tr, 0, \dots, 0) \cdot 
    %     \begin{pmatrix}
    %     0\\[-2mm] \vdots\\[-2mm] 0\\[-2mm] -\mathbf{c}_{k} \\[-2mm] 0 \\[-2mm] \vdots \\[-2mm] 0
    %     \end{pmatrix}
    %  \end{cases}
\end{align}
In particular, if $\epsilon \oline{\epsilon} = +$, $\oline{c}_{ki} c_{kj} \in \bZ_{\geq 0}$, so 
\begin{align*}
    [\epsilon G^{\pm\bs}_{v' \to v_0}]_+^{\bullet k} C^{\pm\bs}_{v_0 \to v} \in 
    \begin{cases}
        \bZ_{\leq 0}^{I \times I} & \mbox{if } (\epsilon, \oline{\epsilon}) = (+, +),\\
        \bZ_{\geq 0}^{I \times I} & \mbox{if } (\epsilon, \oline{\epsilon}) = (-, -).
    \end{cases}
\end{align*}
Using the equation \eqref{eq:FC_decomp_bs} and \eqref{eq:FC_decomp_-bs} repeatedly, we get
\begin{align*}
    F^\bs_{v \to v_0} C^{\bs}_{v_0 \to v} = [\epsilon G^{\bs}_{v' \to v_0}]_+^{\bullet k} C^{\bs}_{v_0 \to v} + 
    % [\epsilon_{\ell-2} G^{\bs}_{v_2 \to v}]_+^{\bullet k_1} C^{\bs}_{v_0 \to v'} +
    \cdots + [\epsilon_{1} G^\bs_{v_1 \to v_0}]^{\bullet k_1}_+ C^\bs_{v_0 \to v_2} + [\epsilon_{0} \mathrm{Id}]_+^{\bullet k_{0}} C^{\bs}_{v_0 \to v_1},\\
    F^\bs_{v \to v_0} C^{-\bs}_{v_0 \to v} = [\oline{\epsilon} G^{-\bs}_{v' \to v_0}]_+^{\bullet k} C^{-\bs}_{v_0 \to v} + 
    % [\epsilon_{\ell-2} G^{\bs}_{v_2 \to v}]_+^{\bullet k_1} C^{\bs}_{v_0 \to v'} +
    \cdots + [\oline{\epsilon}_{1} G^{-\bs}_{v_1 \to v_0}]^{\bullet k_1}_+ C^{-\bs}_{v_0 \to v_2} + [\oline{\epsilon}_{0} \mathrm{Id}]_+^{\bullet k_{0}} C^{-\bs}_{v_0 \to v_1}.
\end{align*}
Since the path $\gamma$ is weakly green, each matrices $[\epsilon_p G^{\bs}_{v_{p} \to v_0}]_+^{\bullet k_p} C^{\bs}_{v_0 \to v_{p+1}}$ and $[\oline{\epsilon}_p G^{-\bs}_{v_p \to v_0}]_+^{\bullet k_p} C^{-\bs}_{v_0 \to v_{p+1}}$ are non-positive for $p = 0, 1, \dots, \ell-1$, so $F^\bs_{v \to v_0} C^{\pm\bs}_{v \to v_0}$ are non-positive.
\end{proof}

\begin{rmk}
By \eqref{eq:[C]C_bs} and \eqref{eq:[C]C_-bs}, we have
\begin{align*}
    [\epsilon G^{\bs}_{v' \to v_0}]_+^{\bullet k} C^{\bs}_{v_0 \to v} = ([\epsilon G^{-\bs}_{v' \to v_0}]_+^{\bullet k} C^{-\bs}_{v_0 \to v})^\tr.
\end{align*}
Thus, 
\begin{align*}
    F^\bs_{v \to v_0} C^{\bs}_{v_0 \to v} = (F^\bs_{v \to v_0} C^{-\bs}_{v_0 \to v})^\tr.
\end{align*}
\end{rmk}
